# Supplementary material for: Constitutive Models for Active Skeletal Muscle: Review, Comparison, and Application in a Novel Continuum Shoulder Model
Source: arXiv:2411.03015 ancillary file (2026-11-30)
Supplement: Supplementary file 1 [file supplements.pdf]

# Supplementary material: Elasticity tensors

## I Active stress approach (ASE)

Considering the isochoric and volumetric contributions in the strain-energy function in Eq. (8), the elasticity tensor is computed to

$$\mathbb{C} = \mathbb{C}_{\mathrm{iso}} + \mathbb{C}_{\mathrm{vol}}. \tag{S1}$$

The volumetric part reads

$$\mathbb{C}_{\mathrm{vol}} = K\left(\mathbf{C}^{-1}\otimes\mathbf{C}^{-1} + 2\ln J\frac{\partial\mathbf{C}^{-1}}{\partial\mathbf{C}}\right) \tag{S2}$$

with

$$\frac{\partial\mathbf{C}^{-1}}{\partial\mathbf{C}}_{ijkl} = -\tfrac{1}{2}\left(C^{-1}_{ik}C^{-1}_{jl} + C^{-1}_{il}C^{-1}_{jk}\right). \tag{S3}$$

The isochoric part is computed using the ficticious elasticity tensor $\bar{\mathbb{C}} = 2J^{-4/3}\frac{\partial\bar{\mathbf{S}}}{\partial\bar{\mathbf{C}}}$ and the modified projection tensor $\tilde{\mathbb{P}} = \mathbf{C}^{-1}\odot\mathbf{C}^{-1} - \frac{1}{3}\mathbf{C}^{-1}\otimes\mathbf{C}^{-1}$ according to the relation

$$\mathbb{C}_{\mathrm{iso}} = \mathbb{P}:\bar{\mathbb{C}}:\mathbb{P}^T + \tfrac{2}{3}J^{-2/3}\left(\bar{\mathbf{S}}:\bar{\mathbf{C}}\right)\tilde{\mathbb{P}} - \tfrac{2}{3}\left(\mathbf{C}^{-1}\otimes\mathbf{S}_{\mathrm{iso}} + \mathbf{S}_{\mathrm{iso}}\otimes\mathbf{C}^{-1}\right). \tag{S4}$$

According to [1, p.272], the ficticious elasticity tensor $\bar{\mathbb{C}}$ for a transversely isotropic material model reads

$$\begin{aligned}\bar{\mathbb{C}} = J^{-4/3}\Bigg\{&\bar{\delta}_1\left(\mathbf{I}\otimes\mathbf{I}\right) + \bar{\delta}_5\left(\mathbf{I}\otimes\mathbf{M} + \mathbf{M}\otimes\mathbf{I}\right) + \bar{\delta}_7\left(\mathbf{M}\otimes\mathbf{M}\right) + \bar{\delta}_8\left(\mathbf{I}\otimes\frac{\partial\bar{I}_5}{\partial\bar{\mathbf{C}}} + \frac{\partial\bar{I}_5}{\partial\bar{\mathbf{C}}}\otimes\mathbf{I}\right)\\ &+ \bar{\delta}_{10}\left(\frac{\partial\bar{I}_5}{\partial\bar{\mathbf{C}}}\otimes\frac{\partial\bar{I}_5}{\partial\bar{\mathbf{C}}}\right) + \bar{\delta}_{11}\left(\mathbf{M}\otimes\frac{\partial\bar{I}_5}{\partial\bar{\mathbf{C}}} + \frac{\partial\bar{I}_5}{\partial\bar{\mathbf{C}}}\otimes\mathbf{M}\right) + \bar{\delta}_{12}\frac{\partial^2\bar{I}_5}{\partial\bar{\mathbf{C}}^2}\Bigg\}\end{aligned} \tag{S5}$$

with the pre-factors

$$\bar{\delta}_1 = -2G_2A_3\bar{I}_4, \qquad \bar{\delta}_5 = 2G_2\left(A_2 - A_3\left(\bar{I}_1 - A_1\right)\right), \qquad \bar{\delta}_8 = 2G_2A_3,$$

$$\bar{\delta}_7 = 24G_1\bar{I}_5\bar{I}_4^{-4} - 2G_2\left(A_3\left(\bar{I}_1 - A_1\right)^2 + A_2\left(2\bar{I}_1 - 3A_1\right)\right)\bar{I}_4^{-1} - 2\bar{I}_4^{-2}\left(\sigma_{\mathrm{f}}^{\mathrm{tot}} - \frac{\partial\sigma_{\mathrm{f}}^{\mathrm{tot}}}{\partial\bar{\lambda}}\bar{I}_4\right),$$

$$\bar{\delta}_{10} = -2G_2A_3\bar{I}_4^{-1}, \qquad \bar{\delta}_{11} = 2G_2\left(A_2 + A_3\left(\bar{I}_1 - A_1\right)\right)\bar{I}_4^{-1} - 8G_1\bar{I}_4^{-3}, \qquad \bar{\delta}_{12} = 4G_1\bar{I}_4^{-2} - 4G_2A_2,$$

and the derivatives

$$\frac{\partial\bar{I}_5}{\partial\bar{\mathbf{C}}} = \mathbf{M}\bar{\mathbf{C}} + \bar{\mathbf{C}}\mathbf{M} \qquad \text{and} \qquad \frac{\partial^2\bar{I}_5}{\partial\bar{\mathbf{C}}^2} = \mathbf{I}\otimes\mathbf{M} + \mathbf{M}\otimes\mathbf{I}.$$

Differentiating $\sigma_{\mathrm{f}}^{\mathrm{tot}}$ with respect to the fiber stretch results in the derivative

$$\frac{\partial\sigma_{\mathrm{f}}^{\mathrm{tot}}}{\partial\bar{\lambda}} = \sigma_{\max}\frac{\partial f_\xi^{\mathrm{p}}}{\partial\bar{\lambda}} + \sigma_{\max}f_{\mathrm{t}}^{\tanh}\frac{\partial f_\xi^{\mathrm{a}}}{\partial\bar{\lambda}} \tag{S6}$$

with the terms

$$\frac{\partial f_\xi^{\mathrm{p}}}{\partial\bar{\lambda}} = \begin{cases} 2D_3\bar{\lambda} + D_4 & \text{if } \bar{\lambda}\geq\lambda_* \\ \bar{\lambda}D_1D_2\mathrm{e}^{D_2\left(\bar{\lambda}-1\right)} + D_1\left(\mathrm{e}^{D_2\left(\bar{\lambda}-1\right)} - 1\right) & \text{if } \lambda_* > \bar{\lambda} > 1 \\ 0 & \text{if } 1\geq\bar{\lambda}, \end{cases} \tag{S7}$$

$$\frac{\partial f_\xi^{\mathrm{a}}}{\partial\bar{\lambda}} = \begin{cases} \frac{1}{\lambda_{\mathrm{opt}}}\left(27\frac{\bar{\lambda}}{\lambda_{\mathrm{opt}}}^2 - 14.4\frac{\bar{\lambda}}{\lambda_{\mathrm{opt}}} + 1.44\right) & \text{if } \bar{\lambda}\leq 0.6\lambda_{\mathrm{opt}} \\ \frac{1}{\lambda_{\mathrm{opt}}}\left(-12\frac{\bar{\lambda}}{\lambda_{\mathrm{opt}}}^2 + 16\frac{\bar{\lambda}}{\lambda_{\mathrm{opt}}} - 3\right) & \text{if } 0.6\lambda_{\mathrm{opt}} < \bar{\lambda} < 1.4\lambda_{\mathrm{opt}} \\ \frac{1}{\lambda_{\mathrm{opt}}}\left(27\frac{\bar{\lambda}}{\lambda_{\mathrm{opt}}}^2 - 57.6\frac{\bar{\lambda}}{\lambda_{\mathrm{opt}}} + 23.04\right) & \text{if } \bar{\lambda}\geq 1.4\lambda_{\mathrm{opt}}. \end{cases} \tag{S8}$$

## II Generalized active strain approach (GASA)

With the strain-energy function in Eq. (16), the material tangent $\mathbb{C}$ reads, as published in [2],

$$\begin{aligned}\mathbb{C} = 2\frac{\partial \mathbf{S}}{\partial \mathbf{C}} = \gamma \Bigg[ &\delta_0 \left(\tilde{\mathbf{L}} + \omega_\mathrm{a}\mathbf{M}\right) \otimes \left(\tilde{\mathbf{L}} + \omega_\mathrm{a}\mathbf{M}\right) + \delta_1 \left(\tilde{\mathbf{L}} + \frac{1+\omega_\mathrm{a}\alpha\lambda^2}{\alpha\lambda^2}\mathbf{M}\right) \otimes \frac{\partial \omega_\mathrm{a}}{\partial \mathbf{C}} \\ &+ \delta_2 \left(\mathbf{C}^{-1}\tilde{\mathbf{L}}\mathbf{C}^{-1} \otimes \mathbf{C}^{-1}\tilde{\mathbf{L}}\mathbf{C}^{-1}\right) + \delta_3 \left(\mathbf{C}^{-1} \otimes \mathbf{C}^{-1}\tilde{\mathbf{L}}\mathbf{C}^{-1} + \mathbf{C}^{-1}\tilde{\mathbf{L}}\mathbf{C}^{-1} \otimes \mathbf{C}^{-1}\right) \\ &+ \delta_4 \mathbf{C}^{-1} \otimes \mathbf{C}^{-1} + \delta_5 \frac{\partial \mathbf{C}^{-1}}{\partial \mathbf{C}} + \delta_6 \frac{\partial \mathbf{C}^{-1}\tilde{\mathbf{L}}\mathbf{C}^{-1}}{\partial \mathbf{C}} \Bigg]\end{aligned} \tag{S9}$$

with the scalar pre-factors

$$\begin{gathered}\delta_0 = \alpha \mathrm{e}^{\alpha(\tilde{I}-1)}, \qquad \delta_1 = \lambda^2 \alpha \mathrm{e}^{\alpha(\tilde{I}-1)}, \qquad \delta_2 = \beta \mathrm{e}^{\beta(\tilde{J}-1)} \det(\mathbf{C})^2, \\ \delta_3 = -(\beta\tilde{J}+1)\mathrm{e}^{\beta(\tilde{J}-1)} \det(\mathbf{C}), \qquad \delta_4 = (\beta\tilde{J}+1)\mathrm{e}^{\beta(\tilde{J}-1)} + \kappa \det(\mathbf{C})^{-\kappa}, \\ \delta_5 = \tilde{J}\mathrm{e}^{\beta(\tilde{J}-1)} - \det(\mathbf{C})^{-\kappa}, \qquad \delta_6 = -\mathrm{e}^{\beta(\tilde{J}-1)} \det(\mathbf{C}).\end{gathered}$$

While the derivative $\frac{\partial \mathbf{C}^{-1}}{\partial \mathbf{C}}$ is given by Eq. (S3), the derivative $\frac{\partial \mathbf{C}^{-1}\tilde{\mathbf{L}}\mathbf{C}^{-1}}{\partial \mathbf{C}}$ is computed to

$$\begin{aligned}\frac{\partial \mathbf{C}^{-1}\tilde{\mathbf{L}}\mathbf{C}^{-1}}{\partial \mathbf{C}}\bigg|_{ijkl} = &-\tfrac{1}{2}\left(C^{-1}_{ik}C^{-1}_{jm}\tilde{L}_{mn}C^{-1}_{nl} + C^{-1}_{il}C^{-1}_{jm}\tilde{L}_{mn}C^{-1}_{nk}\right) \\ &-\tfrac{1}{2}\left(C^{-1}_{jk}C^{-1}_{im}\tilde{L}_{mn}C^{-1}_{nl} + C^{-1}_{jl}C^{-1}_{im}\tilde{L}_{mn}C^{-1}_{nk}\right).\end{aligned} \tag{S10}$$

The derivative of the activation level $\frac{\partial \omega_\mathrm{a}}{\partial \mathbf{C}}$ is obtained as

$$\frac{\partial \omega_\mathrm{a}}{\partial \mathbf{C}} = \frac{1}{2\lambda}\frac{\partial \omega_\mathrm{a}}{\partial \lambda}\mathbf{M} \tag{S11}$$

with

$$\frac{\partial \omega_\mathrm{a}}{\partial \lambda} = \begin{cases} 0 & \text{if } P_\mathrm{a} = 0 \\ \frac{1}{\alpha\lambda^2}\frac{\mathrm{d}W_0(\chi^*)}{\mathrm{d}\lambda} - \frac{2W_0(\chi^*)}{\alpha\lambda^3} - \frac{1}{2\lambda}\tilde{I}''_\mathrm{p} + \frac{1}{2\lambda^2}\tilde{I}'_\mathrm{p} & \text{else.}\end{cases} \tag{S12}$$

While $\tilde{I}'_\mathrm{p}$, the first derivative of the passive part of the first generalized invariant $\tilde{I}_\mathrm{p}$ with respect to $\lambda$, is given by Eq. (32), the second derivative $\tilde{I}''_\mathrm{p}$ reads

$$\tilde{I}''_\mathrm{p} = \frac{\partial^2 \tilde{I}_\mathrm{p}}{\partial \lambda^2} = \tfrac{4}{3}\omega_0\left(\lambda^{-3} - 1\right) + 2. \tag{S13}$$

Differentiation of the Lambert $W$ function with respect to $\lambda$ results in

$$\frac{\mathrm{d}W_0(\chi^*)}{\mathrm{d}\lambda} = \frac{1}{(1+W_0)\,\mathrm{e}^{W_0}}\frac{\mathrm{d}\chi^*}{\mathrm{d}\lambda}.$$

whereby the latter factor is computed to

$$\begin{aligned}\frac{\mathrm{d}\chi^*}{\mathrm{d}\lambda} = &\tfrac{2\alpha}{\gamma}\mathrm{e}^{\frac{\alpha}{2}(2-2\tilde{I}_\mathrm{p}+\lambda\tilde{I}'_\mathrm{p})}\left[P_\mathrm{a} + \lambda\frac{\mathrm{d}P_\mathrm{a}}{\mathrm{d}\lambda} + \tfrac{\alpha}{2}P_\mathrm{a}\lambda\left(\lambda\tilde{I}''_\mathrm{p} - \tilde{I}'_\mathrm{p}\right)\right] \\ &+ \tfrac{2\alpha+\alpha^2}{4}\mathrm{e}^{\frac{\alpha}{2}\lambda\tilde{I}'_\mathrm{p}}\left(\lambda\tilde{I}''_\mathrm{p} + \tilde{I}'_\mathrm{p}\right).\end{aligned} \tag{S14}$$

Under the assumption that the force-velocity dependency $f_\mathrm{v}$ is neglected, the first derivative of $P_\mathrm{a}$ with respect to $\lambda$ is calculated as

$$\frac{\mathrm{d}P_\mathrm{a}}{\mathrm{d}\lambda} = N_\mathrm{a}\sum_{i=1}^{n_\mathrm{MU}} \rho_i F^i_\mathrm{t}\frac{\mathrm{d}f_\xi}{\mathrm{d}\lambda} \tag{S15}$$

with

$$\frac{\mathrm{d}f_\xi}{\mathrm{d}\lambda} = \begin{cases} \frac{(\lambda_\mathrm{min}-\lambda)^2-(\lambda_\mathrm{min}-\lambda_\mathrm{opt})^2}{2(\lambda_\mathrm{min}-\lambda_\mathrm{opt})^3}\exp\left[\frac{(2\lambda_\mathrm{min}-\lambda-\lambda_\mathrm{opt})(\lambda-\lambda_\mathrm{opt})}{2(\lambda_\mathrm{min}-\lambda_\mathrm{opt})^2}\right] & \text{if } \lambda > \lambda_\mathrm{min} \\ 0 & \text{if } \lambda \leqslant \lambda_\mathrm{min}.\end{cases} \tag{S16}$$

## III Active strain approach (ASA)

Based on the strain-energy function in Eq. (23), the elasticity tensor $\mathbb{C}$ contains an elastic and volumetric contribution according to

$$\mathbb{C} = \mathbb{C}_\mathrm{e} + \mathbb{C}_\mathrm{vol}. \tag{S17}$$

Considering the derivative $\frac{\partial \mathbf{C}^{-1}}{\partial \mathbf{C}}$ in Eq. (S3), the volumetric component can be computed to

$$\mathbb{C}_\mathrm{vol} = \gamma \det(\mathbf{C})^{-\kappa} \left( \kappa \mathbf{C}^{-1} \otimes \mathbf{C}^{-1} - \frac{\partial \mathbf{C}^{-1}}{\partial \mathbf{C}} \right). \tag{S18}$$

For simplicity reasons, we use index notation for the complex derivation of the elastic contribution $\mathbb{C}_\mathrm{e}$. Its components are given as

$$\begin{aligned}
\mathbb{C}_{\mathrm{e},ijkl} = 4\det(\mathbf{F}_\mathrm{a}) \Bigg\{ & \left( \frac{\partial \mathbf{F}_\mathrm{a}^{-1}}{\partial \omega_\mathrm{a}} \mathbf{C} \frac{\partial \mathbf{F}_\mathrm{a}^{-1}}{\partial \omega_\mathrm{a}} + {\mathbf{F}_\mathrm{a}}^{-1} \mathbf{C} \frac{\partial^2 \mathbf{F}_\mathrm{a}^{-1}}{\partial \omega_\mathrm{a}^2} \right)_{rs} \mathbf{S}_{\mathrm{e}rs} \frac{\partial \omega_\mathrm{a}}{\partial \mathbf{C}}_{ij} \frac{\partial \omega_\mathrm{a}}{\partial \mathbf{C}}_{kl} \\
& + \left( {\mathbf{F}_\mathrm{a}}^{-1} \mathbf{C} \frac{\partial \mathbf{F}_\mathrm{a}^{-1}}{\partial \omega_\mathrm{a}} \right)_{rs} \mathbf{S}_{\mathrm{e}rs} \frac{\partial^2 \omega_\mathrm{a}}{\partial \mathbf{C}^2}_{ijkl} \\
& + \tfrac{1}{2} \frac{\partial \omega_\mathrm{a}}{\partial \mathbf{C}}_{ij} \left( \frac{\partial \mathbf{F}_\mathrm{a}^{-1}}{\partial \omega_\mathrm{a}} \mathbf{S}_\mathrm{e} {\mathbf{F}_\mathrm{a}}^{-1} + {\mathbf{F}_\mathrm{a}}^{-1} \mathbf{S}_\mathrm{e} \frac{\partial \mathbf{F}_\mathrm{a}^{-1}}{\partial \omega_\mathrm{a}} \right)_{kl} \\
& + \tfrac{1}{2} \left( \frac{\partial \mathbf{F}_\mathrm{a}^{-1}}{\partial \omega_\mathrm{a}} \mathbf{S}_\mathrm{e} {\mathbf{F}_\mathrm{a}}^{-1} + {\mathbf{F}_\mathrm{a}}^{-1} \mathbf{S}_\mathrm{e} \frac{\partial \mathbf{F}_\mathrm{a}^{-1}}{\partial \omega_\mathrm{a}} \right)_{ij} \frac{\partial \omega_\mathrm{a}}{\partial \mathbf{C}}_{kl} \\
& + 2 \left( {\mathbf{F}_\mathrm{a}}^{-1} \mathbf{C} \frac{\partial \mathbf{F}_\mathrm{a}^{-1}}{\partial \omega_\mathrm{a}} \right)_{rs} \frac{\partial \mathbf{S}_\mathrm{e}}{\partial \mathbf{C}_\mathrm{e}}_{rstu} \left( {\mathbf{F}_\mathrm{a}}^{-1} \mathbf{C} \frac{\partial \mathbf{F}_\mathrm{a}^{-1}}{\partial \omega_\mathrm{a}} \right)_{tu} \frac{\partial \omega_\mathrm{a}}{\partial \mathbf{C}}_{ij} \frac{\partial \omega_\mathrm{a}}{\partial \mathbf{C}}_{kl} \\
& + \frac{\partial \omega_\mathrm{a}}{\partial \mathbf{C}}_{ij} {\mathbf{F}_\mathrm{a}}_{kt}^{-1} \left( {\mathbf{F}_\mathrm{a}}^{-1} \mathbf{C} \frac{\partial \mathbf{F}_\mathrm{a}^{-1}}{\partial \omega_\mathrm{a}} \right)_{rs} \frac{\partial \mathbf{S}_\mathrm{e}}{\partial \mathbf{C}_\mathrm{e}}_{rstu} {\mathbf{F}_\mathrm{a}}_{ul}^{-1} \\
& + {\mathbf{F}_\mathrm{a}}_{ir}^{-1} \frac{\partial \mathbf{S}_\mathrm{e}}{\partial \mathbf{C}_\mathrm{e}}_{rstu} \left( {\mathbf{F}_\mathrm{a}}^{-1} \mathbf{C} \frac{\partial \mathbf{F}_\mathrm{a}^{-1}}{\partial \omega_\mathrm{a}} \right)_{tu} {\mathbf{F}_\mathrm{a}}_{sj}^{-1} \frac{\partial \omega_\mathrm{a}}{\partial \mathbf{C}}_{kl} \\
& + \tfrac{1}{2} {\mathbf{F}_\mathrm{a}}_{ir}^{-1} {\mathbf{F}_\mathrm{a}}_{sj}^{-1} \frac{\partial \mathbf{S}_\mathrm{e}}{\partial \mathbf{C}_\mathrm{e}}_{rstu} {\mathbf{F}_\mathrm{a}}_{tk}^{-1} {\mathbf{F}_\mathrm{a}}_{lu}^{-1} \Bigg\}.
\end{aligned} \tag{S19}$$

In the above equation, the elastic stress derivative is computed to

$$\begin{aligned}
\frac{\partial \mathbf{S}_\mathrm{e}}{\partial \mathbf{C}_\mathrm{e}} = \tfrac{1}{2}\gamma \Big[ & \delta_0 \tilde{\mathbf{L}} \otimes \tilde{\mathbf{L}} + \delta_2 \left( \mathbf{C}_\mathrm{e}^{-1} \tilde{\mathbf{L}} \mathbf{C}_\mathrm{e}^{-1} \otimes \mathbf{C}_\mathrm{e}^{-1} \tilde{\mathbf{L}} \mathbf{C}_\mathrm{e}^{-1} \right) + \delta_3 \left( \mathbf{C}_\mathrm{e}^{-1} \otimes \mathbf{C}_\mathrm{e}^{-1} \tilde{\mathbf{L}} \mathbf{C}_\mathrm{e}^{-1} + \mathbf{C}_\mathrm{e}^{-1} \tilde{\mathbf{L}} \mathbf{C}_\mathrm{e}^{-1} \otimes \mathbf{C}_\mathrm{e}^{-1} \right) \\
& + \delta_4 \mathbf{C}_\mathrm{e}^{-1} \otimes \mathbf{C}_\mathrm{e}^{-1} + \delta_5 \frac{\partial \mathbf{C}_\mathrm{e}^{-1}}{\partial \mathbf{C}_\mathrm{e}} + \delta_6 \frac{\partial \mathbf{C}_\mathrm{e}^{-1} \tilde{\mathbf{L}} \mathbf{C}_\mathrm{e}^{-1}}{\partial \mathbf{C}_\mathrm{e}} \Big]
\end{aligned} \tag{S20}$$

with the scalar pre-factors

$$\begin{gathered}
\delta_0 = \alpha \mathrm{e}^{\alpha(\tilde{I}_\mathrm{e}-1)}, \qquad \delta_2 = \beta \mathrm{e}^{\beta(\tilde{J}_\mathrm{e}-1)} \det(\mathbf{C}_\mathrm{e})^2, \qquad \delta_3 = -(\beta \tilde{J}_\mathrm{e} + 1) \mathrm{e}^{\beta(\tilde{J}_\mathrm{e}-1)} \det(\mathbf{C}_\mathrm{e}), \\
\delta_4 = (\beta \tilde{J}_\mathrm{e} + 1) \mathrm{e}^{\beta(\tilde{J}_\mathrm{e}-1)}, \qquad \delta_5 = \tilde{J}_\mathrm{e} \mathrm{e}^{\beta(\tilde{J}_\mathrm{e}-1)}, \qquad \delta_6 = -\mathrm{e}^{\beta(\tilde{J}_\mathrm{e}-1)} \det(\mathbf{C}_\mathrm{e}).
\end{gathered}$$

The second derivative of the activation level $\omega_\mathrm{a}$ in Eq. (S19) reads

$$\frac{\partial^2 \omega_\mathrm{a}}{\partial \mathbf{C}^2} = \frac{1}{4\lambda^3} \left( \lambda \frac{\partial^2 \omega_\mathrm{a}}{\partial \lambda^2} - \frac{\partial \omega_\mathrm{a}}{\partial \lambda} \right) \mathbf{M} \otimes \mathbf{M}. \tag{S21}$$

Due to the implicit formulation of the activation level, the derivatives $\frac{\partial \omega_\mathrm{a}}{\partial \lambda}$ and $\frac{\partial^2 \omega_\mathrm{a}}{\partial \lambda^2}$ are approximated by a central differences scheme. Further, the derivatives of the active deformation gradient and its inverse are given by

$$\frac{\partial^2 \mathbf{F}_\mathrm{a}}{\partial \omega_\mathrm{a}^2} = -\tfrac{3}{4}(1-\omega_\mathrm{a})^{-\frac{5}{2}}\left(\mathbf{I}-\mathbf{M}\right), \tag{S22}$$

$$\frac{\partial \mathbf{F}_\mathrm{a}^{-1}}{\partial \omega_\mathrm{a}} = -{\mathbf{F}_\mathrm{a}}^{-1}\frac{\partial \mathbf{F}_\mathrm{a}}{\partial \omega_\mathrm{a}}{\mathbf{F}_\mathrm{a}}^{-1}, \tag{S23}$$

$$\frac{\partial^2 \mathbf{F}_\mathrm{a}^{-1}}{\partial \omega_\mathrm{a}^2} = -\left(2{\mathbf{F}_\mathrm{a}}^{-1}\frac{\partial \mathbf{F}_\mathrm{a}}{\partial \omega_\mathrm{a}}\frac{\partial \mathbf{F}_\mathrm{a}^{-1}}{\partial \omega_\mathrm{a}} + {\mathbf{F}_\mathrm{a}}^{-1}\frac{\partial^2 \mathbf{F}_\mathrm{a}}{\partial \omega_\mathrm{a}^2}{\mathbf{F}_\mathrm{a}}^{-1}\right). \tag{S24}$$

## IV Modified generalized active strain approach (GASAM)

The material tangent for the GASAM-model is computed by adding the additional term $\mathbb{C}_{\omega_\mathrm{a}}$ to the elasticity tensor $\mathbb{C}$ in Eq. (S9). Based on the additional stress contribution $\mathbf{S}_{\omega_\mathrm{a}}$ in Eq. (25), $\mathbb{C}_{\omega_\mathrm{a}}$ reads

$$\mathbb{C}_{\omega_\mathrm{a}} = 2\frac{\partial \mathbf{S}_{\omega_\mathrm{a}}}{\partial \mathbf{C}} = \tfrac{\gamma}{4}\mathrm{e}^{\alpha(\tilde{I}-1)}\left(\left(\alpha\tilde{I}' + \frac{1}{\lambda}\right)\frac{\partial \omega_\mathrm{a}}{\partial \lambda} + \frac{\partial^2 \omega_\mathrm{a}}{\partial \lambda^2}\right)\mathbf{M}\otimes\mathbf{M} \tag{S25}$$

where

$$\frac{\partial^2 \omega_\mathrm{a}}{\partial \lambda^2} = \frac{1}{\alpha\lambda^2}\left(\frac{6}{\lambda^2}\ln\phi + \frac{1}{\phi}\left(\phi'' - \frac{1}{\phi}\phi'^2 - \frac{4}{\lambda}\phi'\right)\right) \tag{S26}$$

and

$$\phi'' = \frac{\partial^2 \phi}{\partial \lambda^2} = \tfrac{4\alpha^2}{\gamma}\mathrm{e}^{\alpha\left(1-\tilde{I}_\mathrm{p}\right)}P_\mathrm{opt}f_\mathrm{t}^\mathrm{tanh}\left(\left(\alpha\tilde{I}_\mathrm{p}'^2 - \tilde{I}_\mathrm{p}''\right)\int_{\lambda_\mathrm{min}}^{\lambda} f_\xi(\tilde{\lambda})d\tilde{\lambda} - 2f_\xi\tilde{I}_\mathrm{p}' + \tfrac{1}{\alpha}\frac{\mathrm{d}f_\xi}{\mathrm{d}\lambda}\right). \tag{S27}$$

# References


[1] G. A. Holzapfel, *Nonlinear solid mechanics: A continuum approach for engineering*, 1st ed. Chichester: Wiley, 2000.

[2] J. Weickenmeier, M. Itskov, E Mazza, and M. Jabareen, "A physically motivated constitutive model for 3D numerical simulation of skeletal muscles," *International Journal for Numerical Methods in Biomedical Engineering*, vol. 30, no. 5, pp. 545–562, 2014, DOI: 10.1002/cnm.2618.
